# Supplementary material for: Dressed test particles, oscillation centres and pseudo-orbits
Source: arXiv:1107.5201 ancillary file (2011-10-05)
Supplement: Supplementary file 1 [file README.pdf]

## USE OF THE ETA SUBROUTINE

R. L. DEWAR AND D. LEYKAM  
PLASMA RESEARCH LABORATORY, RESEARCH SCHOOL OF PHYSICS AND ENGINEERING  
THE AUSTRALIAN NATIONAL UNIVERSITY  
CANBERRA ACT 0200, AUSTRALIA  
ROBERT.DEWAR@ANU.EDU.AU

### 1. USAGE

This subroutine is to be used accompanied by the following statements in the main program together with the lookup tables in the data files `eo.dat` and `ed.dat`.

```
      REAL E01(17,17),E02(17,17),ED1(17,17),ED2(17,17)
      COMMON/CC/ E01,E02,ED1,ED2
      OPEN(unit=1,file="eo.dat")
      OPEN(unit=2,file="ed.dat")
      DO j=1,17
      READ(1,10) (E01(I,J),I=9,17)
      READ(2,10) (ED1(I,J), I=9,17)
      ENDDO
      DO j=1,17
      READ(1,10) (E02(I,J),I=9,17)
      READ(2,10) (ED2(I,J),I=9,17)
      ENDDO
      CLOSE(1)
      CLOSE(2)
10    FORMAT(F8.6,8F9.6)
```

The subroutine is called by the appearance of the expression `ETA(z)` within an arithmetic expression, where `z` must be a complex variable or a complex arithmetic expression. The type statement `COMPLEX ETA` must appear in the calling program in a position preceding the first use of the function.

This is illustrated in the example program `etaPolarScan.f` provided, which may [1] be compiled and linked by typing on the command line `gfortran -oetaPolarScan etaPolarScan.f`, where the executable `etaPolarScan` is invoked by typing `./etaPolarScan`, producing the output files `etaImPolarScan.txt` and `etaRePolarScan.txt`.

---

*Date:* July 26, 2011.

## 2. LOOKUP TABLES

The data in the files `eo.dat` and `ed.dat` were scanned in from the data listed in [2], which were excerpted and reformatted from [3, Table 5.6], real and imaginary parts of  $ze^z E_1(z)$ , where  $E_1(z)$  is the exponential integral and  $z = x + iy$ :

- `eo.dat` contains the subset  $x = 0(1)16$ , 6D (rows),  $y = 0(1)8$ , 6D (columns), with the first 16 rows being the real parts and the last 16 rows being the imaginary parts;
- `ed.dat` contains the subset  $x = 0(-1)-16$ , 6D (rows),  $y = 0(1)8$ , 6D (columns), with the first 16 rows being the real parts and the last 16 rows being the imaginary parts.

The data in the tables were checked and corrected from tables calculated using the *Mathematica* [4] function `ExpIntegralE[1, z]`. The accuracy of  $\text{ETA}(z)$  was checked using identity (A.5),  $\eta(z) = -if(-iz)$ , where  $f(z)$  is given in *Mathematica* notation by `f[z_] := CosIntegral[z] Sin[z] - (SinIntegral[z] - Pi/2)Cos[z]`.

Subtracting the interpolated values of  $\text{ETA}(z)$  obtained from the output of the example program `etaPolarScan.f` gives the error plot in Fig 1.

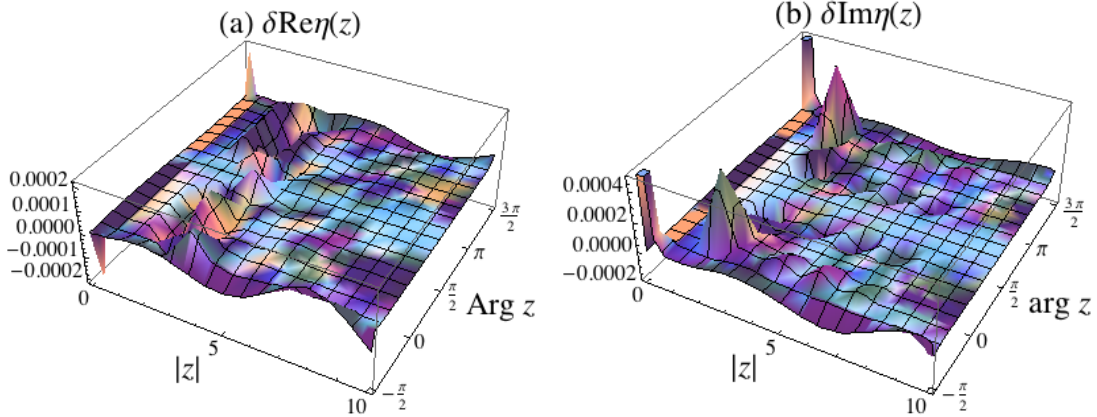

FIGURE 1. Real (a) and imaginary (b) parts of the error  $\delta\eta(z) \equiv \eta(z) - \text{ETA}(z)$ .

## REFERENCES

- [1] The gfortran team 2011 *Using GNU Fortran: For gcc version 4.6.0* Free Software Foundation, Inc. Boston, USA URL <http://gcc.gnu.org/onlinedocs/gfortran.pdf>
- [2] Dewar R L 1967 *Particle-Field Interactions in a Plasma* Master's thesis University of Melbourne
- [3] Abramowitz M and Stegun I A (eds) 1972 *Handbook of Mathematical Functions* 10th ed Applied Mathematics Series - 55 (U.S. Government Printing Office, Washington D.C.: National Bureau of Standards) URL [http://apps.nrbook.com/abramowitz\\_and\\_stegun/index.html](http://apps.nrbook.com/abramowitz_and_stegun/index.html)
- [4] Wolfram Research, Inc 2010 *Mathematica, Version 8* (Champaign, Illinois, USA: Wolfram Research) URL <http://support.wolfram.com/mathematica/reference/general/citing.html>
